# Supplementary material for: Riemannian Denoising Model for Molecular Structure Optimization with Chemical Accuracy
Source: arXiv:2411.19769 source file (2026-01-19)
Supplement: Supplementary file 1 [file Supplementary_Information.pdf]

**Supplementary Information for:**  
**Riemannian Denoising Score Matching for Molecular  
Structure Optimization with Accurate Energy**

Jeheon Woo,<sup>1†</sup> Seonghwan Kim,<sup>1†</sup> Jun Hyeong Kim,<sup>1</sup> and Woo Youn Kim<sup>1,2\*</sup>

<sup>1</sup>*Department of Chemistry, KAIST, 291 Daehak-ro, Yuseong-gu, 34141, Daejeon, Republic of Korea.*

<sup>2</sup>*AI Institute, KAIST, 291 Daehak-ro, Yuseong-gu, 34141, Daejeon, Republic of Korea.*

\*Corresponding author. E-mail: wooyoun@kaist.ac.kr

Contributing authors: woojh@kaist.ac.kr; dmdtka00@kaist.ac.kr; junhkim1226@kaist.ac.kr

<sup>†</sup>*These authors contributed equally to this work.*

# 1 Supplementary results

Supplementary Table 1: **Coverage (COV) and matching (MAT) scores of different methods on the GEOM-QM9 dataset [1].** The recall measurements, COV-R and MAT-R, and the precision measurements, COV-P and MAT-P, are reported as both mean and median values. Three types of initial conformations obtained from ETKDG [2], ConfGF [3], and GeoDiff [4] are evaluated together with their refinements using MMFF and R-DSM.

|                  | COV-R $\delta=0.5$ (%) |        |  | COV-R $\delta=0.25$ (%) |        |  | MAT-R (Å) |        |  | COV-P $\delta=0.25$ (%) |        |  | MAT-P (Å) |        |        |
|------------------|------------------------|--------|--|-------------------------|--------|--|-----------|--------|--|-------------------------|--------|--|-----------|--------|--------|
|                  | Mean                   | Median |  | Mean                    | Median |  | Mean      | Median |  | Mean                    | Median |  | Mean      | Median |        |
| ETKDG            | 84.00                  | 92.06  |  | 49.66                   | 48.58  |  | 0.2963    | 0.2917 |  | 92.51                   | 98.66  |  | 60.71     | 66.41  |        |
| ConfGF           | 89.71                  | 94.35  |  | 52.62                   | 50.45  |  | 0.2675    | 0.2721 |  | 46.50                   | 42.62  |  | 21.65     | 17.55  |        |
| GeoDiff          | 90.52                  | 94.34  |  | 67.25                   | 69.01  |  | 0.2067    | 0.2005 |  | 52.99                   | 51.56  |  | 35.91     | 32.00  |        |
| ETKDG+MMFF       | 81.92                  | 88.52  |  | 61.66                   | 63.77  |  | 0.2599    | 0.2360 |  | 95.51                   | 100.00 |  | 85.80     | 95.83  |        |
| ConfGF+MMFF      | 86.44                  | 90.42  |  | 60.94                   | 60.66  |  | 0.2456    | 0.2400 |  | 54.74                   | 50.83  |  | 39.11     | 37.74  |        |
| GeoDiff+MMFF     | 85.13                  | 89.18  |  | 59.13                   | 60.00  |  | 0.2542    | 0.2485 |  | 53.76                   | 51.25  |  | 38.37     | 36.62  |        |
| ETKDG+R-DSM      | 87.18                  | 93.10  |  | 68.89                   | 68.87  |  | 0.1981    | 0.1808 |  | 95.15                   | 100.00 |  | 86.11     | 93.75  |        |
| ConfGF+R-DSM     | 92.38                  | 95.27  |  | 70.59                   | 73.24  |  | 0.1841    | 0.1760 |  | 52.39                   | 49.54  |  | 35.32     | 30.47  |        |
| GeoDiff+R-DSM    | 90.46                  | 94.04  |  | 70.19                   | 70.83  |  | 0.1853    | 0.1785 |  | 53.98                   | 51.66  |  | 38.99     | 38.20  |        |
| ETKDG+MMFF+R-DSM | 83.43                  | 90.38  |  | 66.00                   | 68.35  |  | 0.2194    | 0.1934 |  | 96.35                   | 100.00 |  | 90.75     | 98.18  |        |
|                  |                        |        |  |                         |        |  |           |        |  |                         |        |  |           | 0.0888 | 0.0622 |

Supplementary Table 2: **Coverage (COV) and matching (MAT) scores of different methods on the ensemble property test set.** The recall measurements, COV-R and MAT-R, and the precision measurements, COV-P and MAT-P, are reported as both mean and median values. Three types of initial conformations obtained from ETKDG [2], ConfGF [3], and GeoDiff [4] are evaluated together with their refinements using MMFF and R-DSM.

|                  | COV-R $\delta=0.5$ (%) |        |       | COV-R $\delta=0.25$ (%) |        |        | MAT-R (Å) |        |       | COV-P $\delta=0.5$ (%) |        |        | COV-P $\delta=0.25$ (%) |        |      | MAT-P (Å) |        |  |
|------------------|------------------------|--------|-------|-------------------------|--------|--------|-----------|--------|-------|------------------------|--------|--------|-------------------------|--------|------|-----------|--------|--|
|                  | Mean                   | Median | Mean  | Mean                    | Median | Mean   | Mean      | Median | Mean  | Mean                   | Median | Mean   | Mean                    | Median | Mean | Mean      | Median |  |
| ETKDG            | 86.89                  | 100.00 | 70.04 | 86.67                   | 0.2354 | 0.1596 | 91.38     | 100.00 | 62.62 | 72                     | 0.2511 | 0.2057 |                         |        |      |           |        |  |
| ConfGF           | 90.75                  | 100.00 | 72.67 | 83.97                   | 0.1965 | 0.1558 | 46.33     | 38.00  | 24.60 | 22                     | 0.5757 | 0.5144 |                         |        |      |           |        |  |
| GeoDiff          | 94.80                  | 100.00 | 73.48 | 71.43                   | 0.1663 | 0.1447 | 48.07     | 44.00  | 27.80 | 22                     | 0.5454 | 0.4721 |                         |        |      |           |        |  |
| ETKDG+MMFF       | 85.98                  | 100.00 | 70.20 | 77.78                   | 0.2465 | 0.2012 | 92.00     | 100.00 | 80.28 | 96                     | 0.1924 | 0.1677 |                         |        |      |           |        |  |
| ConfGF+MMFF      | 88.15                  | 100.00 | 68.16 | 72.08                   | 0.2351 | 0.2063 | 50.07     | 38.00  | 35.20 | 31                     | 0.5251 | 0.4889 |                         |        |      |           |        |  |
| GeoDiff+MMFF     | 86.19                  | 100.00 | 65.10 | 69.05                   | 0.2432 | 0.2133 | 47.73     | 44.00  | 32.80 | 26                     | 0.5324 | 0.4899 |                         |        |      |           |        |  |
| ETKDG+R-DSM      | 89.69                  | 100.00 | 80.58 | 100.00                  | 0.1514 | 0.0649 | 92.83     | 100.00 | 84.14 | 98                     | 0.1404 | 0.0744 |                         |        |      |           |        |  |
| ConfGF+R-DSM     | 83.27                  | 100.00 | 62.02 | 64.58                   | 0.2347 | 0.2132 | 51.54     | 40.83  | 34.78 | 28                     | —      | 0.4984 |                         |        |      |           |        |  |
| GeoDiff+R-DSM    | 96.30                  | 100.00 | 80.19 | 87.08                   | 0.1346 | 0.1066 | 49.40     | 44.00  | 33.87 | 27                     | —      | 0.4597 |                         |        |      |           |        |  |
| ETKDG+MMFF+R-DSM | 85.48                  | 100.00 | 74.62 | 86.67                   | 0.1925 | 0.1279 | 92.07     | 100.00 | 86.07 | 100                    | 0.1286 | 0.0605 |                         |        |      |           |        |  |

Supplementary Table 3: **Comparison of RMSD, D-MAE, and norm distance at  $q$ -coordinates for different models on the QM9 [5] test set.** This table shows root mean square deviation (RMSD), mean absolute error of interatomic distances (D-MAE), and norm distance at  $q$ -coordinates for the predicted structures by MMFF, DSM, R-DSM, and R-DSM\*. R-DSM\* refers to the R-DSM model trained only on noisy structures generated by Euclidean noise-sampling.

|        | RMSD ( $\text{\AA}$ ) |              | D-MAE ( $\text{\AA}$ ) |               | $\ q_0 - \hat{q}_0\ _2$ |               |
|--------|-----------------------|--------------|------------------------|---------------|-------------------------|---------------|
|        | Mean                  | Median       | Mean                   | Median        | Mean                    | Median        |
| MMFF   | 0.200                 | 0.137        | 0.0717                 | 0.0571        | 0.131                   | 0.115         |
| DSM    | 0.166                 | 0.091        | 0.0454                 | 0.0280        | 0.0612                  | 0.0487        |
| R-DSM  | <b>0.104</b>          | <b>0.031</b> | <b>0.0256</b>          | <b>0.0095</b> | <b>0.0269</b>           | <b>0.0119</b> |
| R-DSM* | 0.162                 | 0.087        | 0.0435                 | 0.0257        | 0.0440                  | 0.0286        |

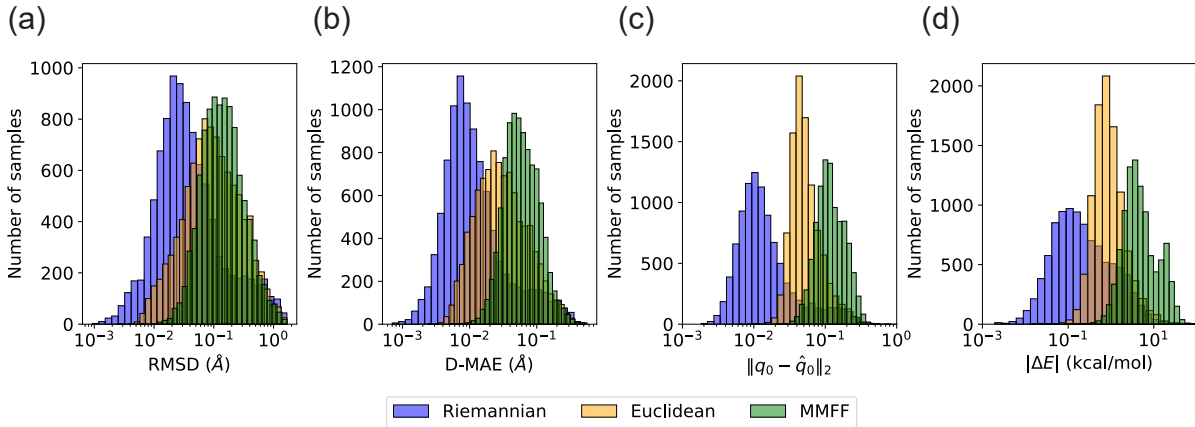

Supplementary Figure 1: **Comparative analysis of molecular structures predicted by R-DSM, DSM, and MMFF.** Histograms compare the distributions of (a) root mean square deviation (RMSD), (b) mean absolute error of interatomic distances (D-MAE), and (c) norm distance at  $q$ -coordinates, and (d) absolute energy difference ( $|\Delta E|$ ); predicted by R-DSM (blue) and DSM (yellow) models and MMFF (green). The sampling was performed on the QM9 [5] set, and the energy values were obtained from single point DFT calculations.

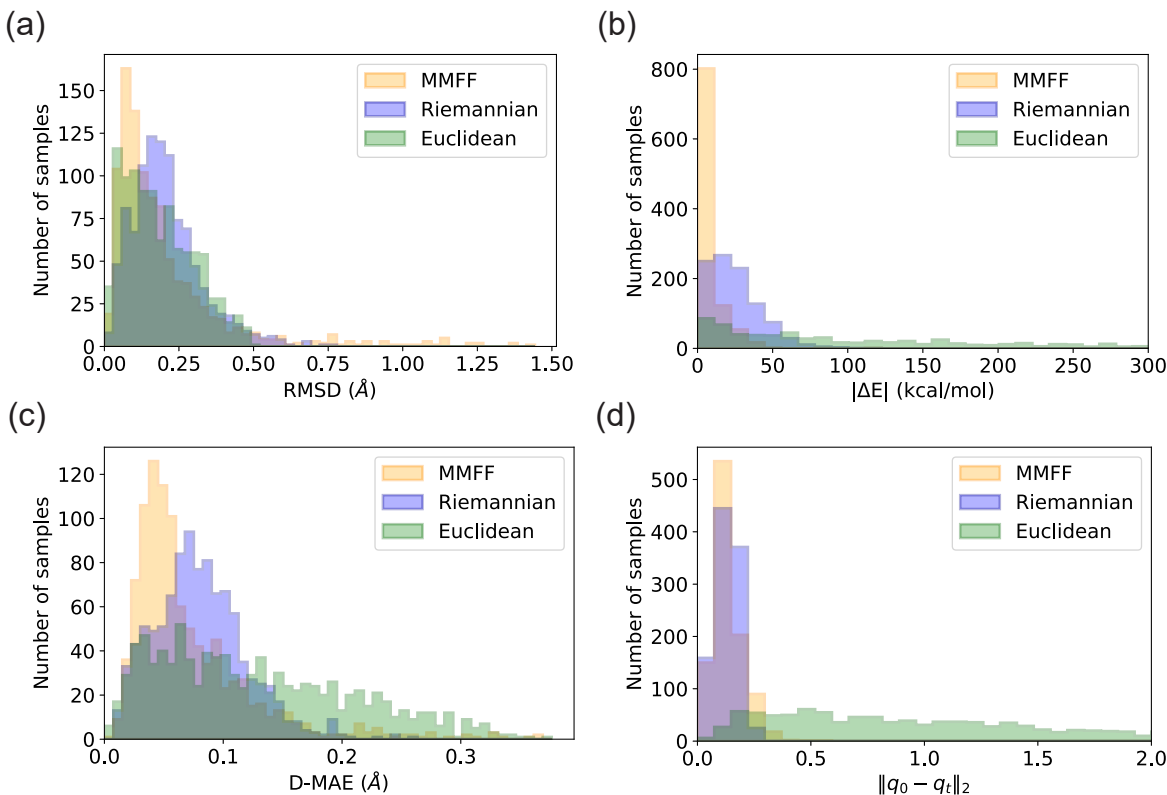

Supplementary Figure 2: **Comparison of molecular structures sampled from noisy distributions of Euclidean and Riemannian spaces.** The distributions of (a) RMSD, (b) absolute energy difference  $|\Delta E|$ , (c) mean absolute error of interatomic distances (D-MAE), and (d) norm distance at  $q$ -coordinates; for molecular structures obtained by MMFF (orange), Riemannian noise-sampling (blue), and Euclidean noise-sampling (green), with the DFT structures as reference. Each distribution is plotted with 1,000 randomly selected molecules for each method; however, 23 samples are excluded from the Euclidean noise-sampled structures due to failure to converge in the SCF calculation.

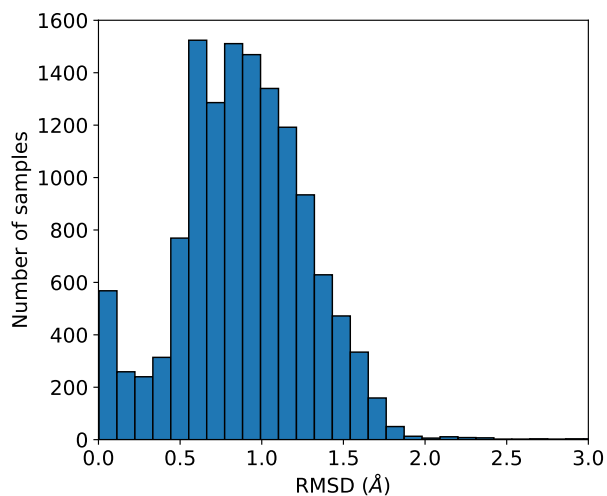

Supplementary Figure 3: **Distribution of RMSD between reference conformations of the GEOM-QM9 [1] test set.**

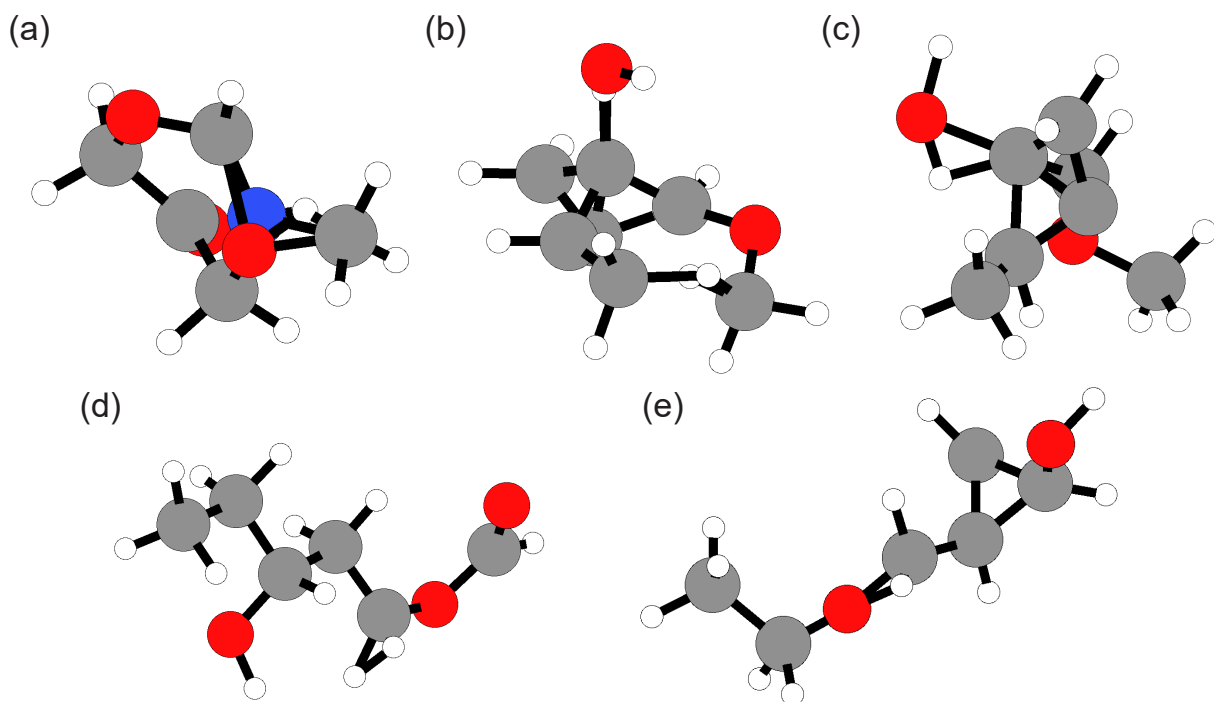

Supplementary Figure 4: **Visualization of starting structures diverged in refinement using R-DSM.** (a) and (b) show the starting structures obtained by ConfGF, while (c) presents the starting structure from GeoDiff. (d) and (e) show the starting structures from ETKDG. Extremely short bond lengths or collapsing structures can be observed.

## 2 Training details

This section outlines the training details for R-DSM. The loss function of R-DSM is defined as:

$$\mathcal{L}(\theta) = \mathbb{E}_{\mathbb{P}} \left[ \int_0^{t_{\max}} \sigma_t^2 \left\| s_{\theta}(X_t, t) - \frac{\exp_{X_t}^{-1}(X_0)}{\sigma_t^2} \right\|_g^2 dt \right]. \quad (1)$$

By reformulating  $s_{\theta}$  with  $f_{\theta}/\sigma_t^2$ , Eq. 1 becomes

$$\mathcal{L}(\theta) = \mathbb{E}_{\mathbb{P}} \left[ \int_0^{t_{\max}} \frac{1}{\sigma_t^2} \left\| f_{\theta}(X_t) - \exp_{X_t}^{-1}(X_0) \right\|_g^2 dt \right]. \quad (2)$$

Thus, the neural network  $f_{\theta}(X_t)$  is trained to predict  $\exp_{X_t}^{-1}(X_0)$ , the direction vector on the tangent plane.

To train the R-DSM model efficiently, we adopted a two-step approach. Initially, R-DSM was pretrained using noisy structures generated through Euclidean noise-sampling, which can be obtained immediately. This was followed by fine-tuning using noisy structures obtained from Riemannian noise-sampling.

During pretraining, we approximate the logarithmic map  $\exp_{x_t}^{-1}(x_0)$  for computational efficiency as follows:

$$\exp_{x_t}^{-1}(x_0) \approx \frac{\text{Proj}_{T_{x_t}\mathcal{M}}(q_0 - q_t)}{\|\text{Proj}_{T_{x_t}\mathcal{M}}(q_0 - q_t)\|_2} \|q_0 - q_t\|_2, \quad (3)$$

where  $q_t$  and  $q_0$  denotes the vector of  $q$ -coordinate in  $\mathbb{R}^{|\mathcal{E}|}$  corresponding to  $x_t$  and  $x_0$ , respectively, and  $\text{Proj}_{T_{x_t}\mathcal{M}}$  represents the projection of  $(q_0 - q_t)$  onto the tangent plane at  $q_t$  which is subspace of  $\mathbb{R}^{|\mathcal{E}|}$ . The size relationship among the three vectors is as follows:  $\|\exp_{x_t}^{-1}(x_0)\|_g \geq \|q_0 - q_t\|_2 \geq \|\text{Proj}_{T_{x_t}\mathcal{M}}(q_0 - q_t)\|_2$ . To correct the reduction in length due to projection, we rescale the vector to match  $\|q_0 - q_t\|_2$ . Accurately computing  $\exp_{x_t}^{-1}(x_0)$ , by determining the geodesic path between  $x_0$  and  $x_t$  on the manifold and obtaining the associated tangent vector, involves a non-negligible computational cost. For efficiency, this approximation is applied instead.

As described in the main text, the noisy structure  $x_t$  in Riemannian space is obtained as follows:

$$x_t = \exp_{x_0}(\sigma_t \varepsilon_t), \quad (4)$$

where  $\varepsilon_t \in T_{x_0}\mathcal{M}$  is a tangent vector representing the direction of noise. In our implementation, the diffusion process is simulated by sampling velocity vectors within the tangent space  $T_{x_t}\mathcal{M}$  to represent small incremental changes. These sampled tangent vectors are then mapped back onto the manifold via the exponential map  $\exp_{x_t}$ , effectively solving the geodesic equation with the initial velocity provided by the sample. We use the Runge-Kutta method to discretize and solve Eq. 4 numerically. For efficiency, noisy structures were pre-generated and stored for use in the training phase, with three noisy structures for each reference structure in QM9 [5] and one for each in GEOM-QM9 [1].

Details on hyperparameters related to DSM and R-DSM can be found in Supplementary Table 4.

Supplementary Table 4: **Hyperparameters of R-DSM and DSM.**

| parameter         | R-DSM   | DSM     |
|-------------------|---------|---------|
| $\beta_1$         | 1e-7    | 1e-7    |
| $\beta_T$         | 2e-3    | 2e-3    |
| $\beta$ scheduler | sigmoid | sigmoid |
| $T$               | 5,000   | 5,000   |
| $t_{\max}$        | 1,500   | 5,000   |
| hidden dimension  | 128     | 128     |
| layers            | 7       | 7       |
| activation        | swish   | swish   |
| batch size        | 300     | 300     |
| epoch             | 3,000   | 3,000   |
| sampling method   | ODE     | ODE     |
| sampling steps    | 128     | 128     |

### 3 Performance and the number of function evaluations

This section examines the performance of DSM and R-DSM models in terms of convergence of accuracy and computational efficiency as a function of the number of function evaluations (nfe).

In Supplementary Figure 5, convergence of accuracy is analyzed by plotting various measurements (RMSD, D-MAE, and  $\|q_0 - \hat{q}_0\|_2$ ) as a function of nfe. R-DSM<sup>†</sup> demonstrates stable accuracy even at low nfe values, indicating that the model maintains robustness with fewer function evaluations. Both DSM and R-DSM<sup>†</sup> converge across all three measurements by nfe=128.

Compared to DSM, R-DSM<sup>†</sup> requires exponential mapping, which introduces additional computational cost. Given the trade-off between performance convergence and inference time, selecting an appropriate nfe is crucial for efficiency. When nfe is sufficiently large, the denoising of molecular structures on the manifold can be approximated in smaller, linear segments, allowing the tangent vectors to be applied in Euclidean space without the need for exponential mapping.

To explore this further, we evaluate R-DSM without exponential mapping at nfe=16 and 128, comparing its accuracy and computational efficiency with R-DSM<sup>†</sup> (see Supplementary Table 5). The results show that R-DSM achieves nearly equivalent performance to R-DSM<sup>†</sup> at nfe=128, while being approximately five times faster. Therefore, in evaluations in the main text, we used DSM and R-DSM with nfe=128.

Supplementary Table 5: **Elapsed CPU time per sample and comparison of RMSD, D-MAE, and norm distance at  $q$ -coordinates for DSM and R-DSM models with the number of function evaluations (nfe) of 16 and 128.** Sampling for the two R-DSM models was performed both with and without exponential mapping, referred to as R-DSM<sup>†</sup> and R-DSM, respectively. This table shows the root mean square deviation (RMSD), mean absolute error of interatomic distances (D-MAE), and norm distance at  $q$ -coordinates ( $\|q_0 - \hat{q}_0\|_2$ ) for the predicted structures by DSM, R-DSM, and R-DSM<sup>†</sup> at two different levels of function evaluations. Elapsed times were measured using 16 threads on a computing node equipped with Intel(R) Xeon(R) Gold 6326 CPUs (2.90 GHz) and a batch size of 300.

| Method                       | RMSD (Å) |        | D-MAE (Å) |         | $\ q_0 - \hat{q}_0\ _2$ |        | Time    |
|------------------------------|----------|--------|-----------|---------|-------------------------|--------|---------|
|                              | Mean     | Median | Mean      | Median  | Mean                    | Median |         |
| DSM (nfe=16)                 | 0.180    | 0.0971 | 0.0572    | 0.0302  | 0.0901                  | 0.0510 | 0.046 s |
| R-DSM <sup>†</sup> (nfe=16)  | 0.109    | 0.0334 | 0.0270    | 0.00996 | 0.0273                  | 0.0124 | 0.31 s  |
| R-DSM (nfe=16)               | 0.109    | 0.0335 | 0.0270    | 0.00999 | 0.0299                  | 0.0130 | 0.070 s |
| DSM (nfe=128)                | 0.166    | 0.0911 | 0.0454    | 0.0280  | 0.0612                  | 0.0487 | 0.32 s  |
| R-DSM <sup>†</sup> (nfe=128) | 0.104    | 0.0315 | 0.0256    | 0.00952 | 0.0259                  | 0.0118 | 2.40 s  |
| R-DSM (nfe=128)              | 0.104    | 0.0314 | 0.0256    | 0.00951 | 0.0269                  | 0.0119 | 0.55 s  |

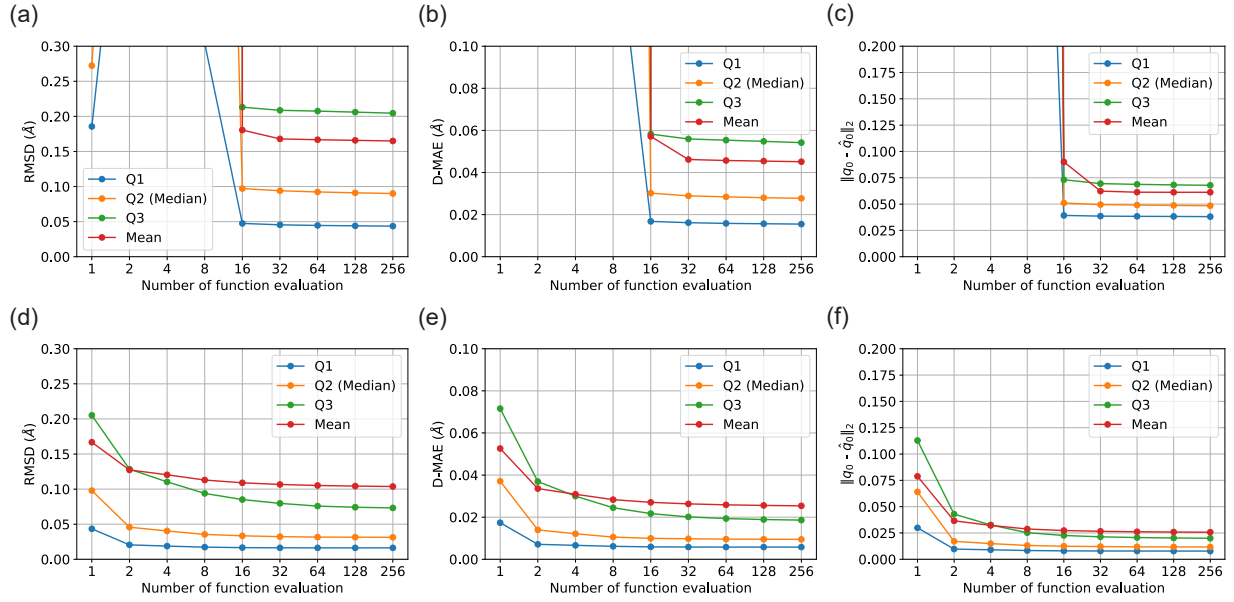

Supplementary Figure 5: **Convergence analysis of different measurements based on the number of function evaluations.** (a)-(c) represent results obtained from DSM, while (d)-(f) correspond to R-DSM<sup>†</sup> with exponential mapping. The measurements plotted include root mean square deviation (RMSD), mean absolute error of interatomic distances (D-MAE), and norm distance as a function of the number of function evaluations. Each subfigure shows the distribution of performance across different quartiles (Q1, Q2, Q3) and the mean.

## Supplementary References

- [1] S. Axelrod and R. Gomez-Bombarelli, "Geom, energy-annotated molecular conformations for property prediction and molecular generation," *Scientific Data* **9**, 185 (2022).
- [2] S. Riniker and G. A. Landrum, "Better informed distance geometry: using what we know to improve conformation generation," *Journal of chemical information and modeling* **55**, 2562–2574 (2015).
- [3] C. Shi, S. Luo, M. Xu, and J. Tang, "Learning gradient fields for molecular conformation generation," (2021).
- [4] M. Xu, L. Yu, Y. Song, C. Shi, S. Ermon, and J. Tang, "Geodiff: a geometric diffusion model for molecular conformation generation," (2022).
- [5] R. Ramakrishnan, P. O. Dral, M. Rupp, and O. A. Von Lilienfeld, "Quantum chemistry structures and properties of 134 kilo molecules," *Scientific data* **1**, 1–7 (2014).
